# Supplementary material for: Investigation of the spin dynamics of quantum spin dimers with Dzyaloshinsky-Moriya interaction
Source: arXiv:2505.11088 source file (2025-05-16)
Supplement: Supplementary file 1 [file Supplement.pdf]

# Supplementary Material to "Investigation of the spin dynamics of quantum spin dimers with Dzyaloshinsky-Moriya interaction"

R. Wieser[1,2], R. Sanchez Galan[3]

*1. School of Physics and Optoelectronic Engineering,*

*Nanjing University of Information Science and Technology, Nanjing 210044, China*

*2. Jiangsu Key Laboratory for Optoelectronic Detection of Atmosphere and Ocean,*

*Nanjing University of Information Science and Technology, Nanjing 210044, China*

*3. 4i Intelligent Insights, Tecnoincubadora Marie Curie,*

*PCT Cartuja, 41092 Sevilla, Spain*

(Dated: March 2, 2025)

PACS numbers: 75.50.Ee, 75.50.Gg, 75.10.Jm

The descriptions in the supplementary material are independent of the actual manuscript and are unnecessary to understand the manuscript.

## I. EIGENENERGIES AND EIGENSTATES OF THE SPIN DIMER

The Hamilton operator H of the spin dimer in local coordinates is given as:

$$\mathrm{H} = -\tilde{J}(\vec{S}_1 \cdot \vec{S}_2) + J_x S_1^x S_2^x - B_1 S_1^z \ , \tag{1}$$

and the corresponding matrix as:

$$\mathrm{H} = \begin{pmatrix} -\tilde{J} - B_1 & 0 & 0 & -J_x \\ 0 & \tilde{J} - B_1 & J_x - 2\tilde{J} & 0 \\ 0 & J_x - 2\tilde{J} & \tilde{J} + B_1 & 0 \\ -J_x & 0 & 0 & -\tilde{J} + B_1 \end{pmatrix} . \tag{2}$$

The parameters $\tilde{J}$ and $J_x$ correspond to the strength of the exchange interaction and exchange anisotropy in local coordinates. $B_1$ is the external magnetic field, as described in detail in the manuscript.

Exact diagonalization delivers the following eigenenergies $E_n$ and eigenstates $|\varphi_n\rangle$:

$$\begin{aligned}
E_1 &= -\sqrt{J_x^2 + B_1^2} - \tilde{J} \ , & |\varphi_1\rangle &= \left(1, 0, 0, +\tfrac{\sqrt{J_x^2+B_1^2}-B_1}{J_x}\right)^{\mathrm{T}} \\
E_2 &= +\sqrt{J_x^2 + B_1^2} - \tilde{J} \ , & |\varphi_2\rangle &= \left(1, 0, 0, -\tfrac{\sqrt{J_x^2+B_1^2}+B_1}{J_x}\right)^{\mathrm{T}} \\
E_3 &= \tilde{J} - \sqrt{J_x^2 - 4\tilde{J}J_x + 4\tilde{J}^2 + B_1^2} \ , & |\varphi_3\rangle &= \left(0, 1, \tfrac{B_1-\sqrt{J_x^2-4\tilde{J}J_x+4\tilde{J}^2+B_1^2}}{J_x-2\tilde{J}}, 0\right)^{\mathrm{T}} \\
E_4 &= \tilde{J} + \sqrt{J_x^2 - 4\tilde{J}J_x + 4\tilde{J}^2 + B_1^2} \ , & |\varphi_4\rangle &= \left(0, 1, \tfrac{B_1+\sqrt{J_x^2-4\tilde{J}J_x+4\tilde{J}^2+B_1^2}}{J_x-2\tilde{J}}, 0\right)^{\mathrm{T}}
\end{aligned}$$

Please notice that the given eigenstates $|\varphi_n\rangle$ are not normalized. The normalized eigenstates are

$$|\psi_n\rangle = \frac{|\varphi_n\rangle}{||\langle\varphi_n|\varphi_n\rangle||} \ , \tag{4}$$

where $||\ldots||$ stands for the norm.

The corresponding limits $B_1 \to \pm\infty$, and the special case $B_1 = 0$ (all normalized) are:

- $B_1 = 0$ :

$$E_1 = -J_x - \tilde{J}\ , \quad |\psi_1\rangle = \tfrac{1}{\sqrt{2}}\,(1,0,0,1)^{\mathrm{T}}$$
$$E_2 = +J_x - \tilde{J}\ , \ |\psi_2\rangle = \tfrac{1}{\sqrt{2}}\,(1,0,0,-1)^{\mathrm{T}}$$
$$E_3 = 3\tilde{J} - J_x\ , \ |\psi_3\rangle = \tfrac{1}{\sqrt{2}}\,(0,1,-1,0)^{\mathrm{T}}$$
$$E_4 = +J_x - \tilde{J}\ , \quad |\psi_4\rangle = \tfrac{1}{\sqrt{2}}\,(0,1,1,0)^{\mathrm{T}}$$

- $B_1 \to +\infty$ :

$$E_1 = -B_1\ , \quad |\psi_1\rangle = (1,0,0,0)^{\mathrm{T}}$$
$$E_2 = +B_1\ , \ |\psi_2\rangle = (0,0,0,-1)^{\mathrm{T}}$$
$$E_3 = -B_1\ , \quad |\psi_3\rangle = (0,1,0,0)^{\mathrm{T}}$$
$$E_4 = +B_1\ , \quad |\psi_4\rangle = (0,0,1,0)^{\mathrm{T}}$$

- $B_1 \to -\infty$ :

$$E_1 = -B_1\ , \quad |\psi_1\rangle = (0,0,0,1)^{\mathrm{T}}$$
$$E_2 = +B_1\ , \quad |\psi_2\rangle = (1,0,0,0)^{\mathrm{T}}$$
$$E_3 = -B_1\ , \ |\psi_3\rangle = (0,0,-1,0)^{\mathrm{T}}$$
$$E_4 = +B_1\ , \quad |\psi_4\rangle = (0,1,0,0)^{\mathrm{T}}$$

## II. GENERAL SOLUTION OF THE DYNAMICS OF THE SPIN DIMER

The following description is in local coordinates. When we assume that the Hamilton operator:

$$\mathrm{H} = -\tilde{J}\vec{S}_1 \cdot \vec{S}_2 + J_x S_1^x S_2^x - B_1 S_1^z\ , \tag{8}$$

describes the spin spiral dimer, and the initial quantum state $|\psi(t=0)\rangle$ is a superposition of the two classical spiral states $|\uparrow\uparrow\rangle$ and $|\downarrow\downarrow\rangle$

$$|\psi(t=0)\rangle = \cos\vartheta\,|\uparrow\uparrow\rangle + \sin\vartheta\, e^{i\varphi}\,|\downarrow\downarrow\rangle\ , \tag{9}$$

then, the dynamics are described by the ket:

$$
|\psi(t)\rangle \;=\; e^{\frac{i\tilde{J}t}{\hbar}} \left\{ \left[ \cos\left(\frac{\sqrt{J_x^2+B_1^2}}{\hbar}t\right)\cos\vartheta + \frac{i\sin\left(\frac{\sqrt{J_x^2+B_1^2}}{\hbar}t\right)\left(B_1\cos\vartheta - J_x\sin\vartheta\, e^{i\varphi}\right)}{\sqrt{J_x^2+B_1^2}} \right] |\uparrow\uparrow\rangle \right.
$$

$$
\left. + \left[ \cos\left(\frac{\sqrt{J_x^2+B_1^2}}{\hbar}t\right)\sin\vartheta\, e^{i\varphi} - \frac{i\sin\left(\frac{\sqrt{J_x^2+B_1^2}}{\hbar}t\right)\left(B_1\sin\vartheta\, e^{i\varphi} + J_x\cos\vartheta\right)}{\sqrt{J_x^2+B_1^2}} \right] |\downarrow\downarrow\rangle \right\} . \tag{10}
$$

$|\psi(t)\rangle$ is the result of solving the time-dependent Schrödinger equation, considering the Hamilton operator H and the above given initial quantum state $|\psi(t=0)\rangle$. The parameters $\vartheta$ and $\varphi$ set the initial state. Please note the similarity of the initial state to the description of a single spin $S = 1/2$ using the Bloch sphere. Once $|\psi(t)\rangle$ is known, the spin expectation values and the time dependence of the energy can be explicitly calculated:

$$
\langle S_{1,2}^{x,y}(t)\rangle \;=\; \langle\psi(t)|S_{1,2}^{x,y}(t)|\psi(t)\rangle = 0 \,, \tag{11a}
$$

$$
\begin{aligned}
\langle S_{1,2}^{z}(t)\rangle \;=\; & \frac{J_x\sin(2\vartheta)\,\sin\varphi\,\sin\left(\frac{2\sqrt{J_x^2+B_1^2}}{\hbar}t\right)}{\sqrt{J_x^2+B_1^2}} - \frac{2B_1J_x\sin(2\vartheta)\,\cos\varphi\,\sin^2\left(\frac{\sqrt{J_x^2+B_1^2}}{\hbar}t\right)}{J_x^2+B_1^2} \\
& + \frac{(B_1^2-J_x^2)\cos(2\vartheta)\,\sin^2\left(\frac{\sqrt{J_x^2+B_1^2}}{\hbar}t\right)}{J_x^2+B_1^2} + \cos(2\vartheta)\,\cos^2\left(\frac{\sqrt{J_x^2+B_1^2}}{\hbar}t\right) \,,
\end{aligned} \tag{11b}
$$

and

$$
E = \langle\psi(t)|\mathrm{H}|\psi(t)\rangle = J_x\sin(2\vartheta)\,\cos\varphi - B_1\cos(2\vartheta) - \tilde{J} \,. \tag{12}
$$

Finally, two remarks:

1. The spin expectation values $\langle S_{1,2}^{x,y,z}\rangle$ are identical because of the use of local coordinates. In local coordinates, both spins are parallel aligned along the $z$-axis. The dynamics in global coordinates occur after a transformation (rotations) back to the global coordinates.

2. The energy $E$ is time-independent.

## III. TRANSFORMATION FROM LOCAL TO GLOBAL COORDINATES

The transformation from local to global coordinates or in the opposite direction occurs via spin rotation. The Hamilton operator $\tilde{\mathrm{H}}$ transforms in a similar way as described for the classical spin spiral in [1]. The only difference is that here, we assume that the first spin is in both coordinates in the $z$-direction, and only the second spin rotates according to the vector of the Dzyaloshinsky-Moriya interaction.

The quantum states transfer, as any quantum mechanics textbook describes. The difference here is that the spin operators act on a single spin of a two-spin system. So our operators are:

$$\sigma_1^{x,y,z} = \sigma_{x,y,z} \otimes \hat{1} \ , \tag{13a}$$

$$\sigma_2^{x,y,z} = \hat{1} \otimes \sigma_{x,y,z} \ . \tag{13b}$$

Here, the $\sigma_{x,y,z}$ are the Pauli matrices, and $\hat{1}$ is the $2 \times 2$ unit matrix.

With these expressions, we can write the rotations given by the rotation operators $R_n^\eta(\theta)$,

with $n \in \{1,2\}$ and $\eta \in \{x,y,z\}$, as:

$$R_1^x(\theta) = e^{i\frac{\theta}{2}\sigma_1^x} = \begin{pmatrix} \cos\frac{\theta}{2} & 0 & i\sin\frac{\theta}{2} & 0 \\ 0 & \cos\frac{\theta}{2} & 0 & i\sin\frac{\theta}{2} \\ i\sin\frac{\theta}{2} & 0 & \cos\frac{\theta}{2} & 0 \\ 0 & i\sin\frac{\theta}{2} & 0 & \cos\frac{\theta}{2} \end{pmatrix}, \tag{14a}$$

$$R_2^x(\theta) = e^{i\frac{\theta}{2}\sigma_2^x} = \begin{pmatrix} \cos\frac{\theta}{2} & i\sin\frac{\theta}{2} & 0 & 0 \\ i\sin\frac{\theta}{2} & \cos\frac{\theta}{2} & 0 & 0 \\ 0 & 0 & \cos\frac{\theta}{2} & i\sin\frac{\theta}{2} \\ 0 & 0 & i\sin\frac{\theta}{2} & \cos\frac{\theta}{2} \end{pmatrix}, \tag{14b}$$

$$R_1^y(\theta) = e^{i\frac{\theta}{2}\sigma_1^y} = \begin{pmatrix} \cos\frac{\theta}{2} & 0 & \sin\frac{\theta}{2} & 0 \\ 0 & \cos\frac{\theta}{2} & 0 & \sin\frac{\theta}{2} \\ -\sin\frac{\theta}{2} & 0 & \cos\frac{\theta}{2} & 0 \\ 0 & -\sin\frac{\theta}{2} & 0 & \cos\frac{\theta}{2} \end{pmatrix}, \tag{14c}$$

$$R_2^y(\theta) = e^{i\frac{\theta}{2}\sigma_2^y} = \begin{pmatrix} \cos\frac{\theta}{2} & \sin\frac{\theta}{2} & 0 & 0 \\ -\sin\frac{\theta}{2} & \cos\frac{\theta}{2} & 0 & 0 \\ 0 & 0 & \cos\frac{\theta}{2} & \sin\frac{\theta}{2} \\ 0 & 0 & -\sin\frac{\theta}{2} & \cos\frac{\theta}{2} \end{pmatrix}, \tag{14d}$$

$$R_1^z(\theta) = e^{i\frac{\theta}{2}\sigma_1^z} = \begin{pmatrix} e^{+i\frac{\theta}{2}} & 0 & 0 & 0 \\ 0 & e^{+i\frac{\theta}{2}} & 0 & 0 \\ 0 & 0 & e^{-i\frac{\theta}{2}} & 0 \\ 0 & 0 & 0 & e^{-i\frac{\theta}{2}} \end{pmatrix}, \tag{14e}$$

$$R_2^z(\theta) = e^{i\frac{\theta}{2}\sigma_2^z} = \begin{pmatrix} e^{+i\frac{\theta}{2}} & 0 & 0 & 0 \\ 0 & e^{-i\frac{\theta}{2}} & 0 & 0 \\ 0 & 0 & e^{+i\frac{\theta}{2}} & 0 \\ 0 & 0 & 0 & e^{-i\frac{\theta}{2}} \end{pmatrix}. \tag{14f}$$

These operators describe the effect of a rotation around the $\eta$-axis, with rotation angle $\theta$ acting on the first, respectively, second spin of a quantum state. In particular, the action of

$R_2^y(\theta)$ on the two classical spiral states, in local coordinates, is given by:

$$\begin{aligned} R_2^x(\theta)|\uparrow\uparrow\rangle &= \begin{pmatrix} \cos\frac{\theta}{2} & i\sin\frac{\theta}{2} & 0 & 0 \\ i\sin\frac{\theta}{2} & \cos\frac{\theta}{2} & 0 & 0 \\ 0 & 0 & \cos\frac{\theta}{2} & i\sin\frac{\theta}{2} \\ 0 & 0 & i\sin\frac{\theta}{2} & \cos\frac{\theta}{2} \end{pmatrix} \begin{pmatrix} 1 \\ 0 \\ 0 \\ 0 \end{pmatrix} = \begin{pmatrix} \cos\frac{\theta}{2} \\ i\sin\frac{\theta}{2} \\ 0 \\ 0 \end{pmatrix} \\ &= \cos\frac{\theta}{2}|\uparrow\uparrow\rangle + i\sin\frac{\theta}{2}|\uparrow\downarrow\rangle = |\uparrow\nearrow\rangle \,, \end{aligned} \tag{15a}$$

$$\begin{aligned} R_2^x(\theta)|\downarrow\downarrow\rangle &= \begin{pmatrix} \cos\frac{\theta}{2} & i\sin\frac{\theta}{2} & 0 & 0 \\ i\sin\frac{\theta}{2} & \cos\frac{\theta}{2} & 0 & 0 \\ 0 & 0 & \cos\frac{\theta}{2} & i\sin\frac{\theta}{2} \\ 0 & 0 & i\sin\frac{\theta}{2} & \cos\frac{\theta}{2} \end{pmatrix} \begin{pmatrix} 0 \\ 0 \\ 0 \\ 1 \end{pmatrix} = \begin{pmatrix} 0 \\ 0 \\ i\sin\frac{\theta}{2} \\ \cos\frac{\theta}{2} \end{pmatrix} \\ &= i\sin\frac{\theta}{2}|\downarrow\uparrow\rangle + \cos\frac{\theta}{2}|\downarrow\downarrow\rangle = |\downarrow\swarrow\rangle \,. \end{aligned} \tag{15b}$$

If we take as an example the quantum state in local coordinates

$$|\psi(t)\rangle = e^{\frac{i\tilde{J}t}{\hbar}} \left[\cos\left(\frac{J_x t}{\hbar}\right)|\uparrow\uparrow\rangle - i\sin\left(\frac{J_x t}{\hbar}\right)|\downarrow\downarrow\rangle\right] \,, \tag{16}$$

which occurs during the oscillatory dynamics when the initial quantum state is the spin spiral state $|\psi(t=0)\rangle = |\uparrow\uparrow\rangle$, we can transfer this state into global coordinates:

$$|\Psi(t)\rangle = R_2^y(\theta)|\psi(t)\rangle \;=\; e^{\frac{i\tilde{J}t}{\hbar}} \left[\cos\left(\frac{J_x t}{\hbar}\right) R_2^y(\theta)|\uparrow\uparrow\rangle - i\sin\left(\frac{J_x t}{\hbar}\right) R_2^y(\theta)|\downarrow\downarrow\rangle\right] \,. \tag{17}$$

The above leads to:

$$|\Psi(t)\rangle = e^{\frac{i\tilde{J}t}{\hbar}} \left[\cos\left(\frac{J_x t}{\hbar}\right)|\uparrow\nearrow\rangle - i\sin\left(\frac{J_x t}{\hbar}\right)|\downarrow\swarrow\rangle\right] \,, \tag{18}$$

as well as,

$$\begin{aligned} |\Psi(t)\rangle &= e^{\frac{i\tilde{J}t}{\hbar}} \Bigg[\cos\left(\frac{J_x t}{\hbar}\right)\cos\frac{\theta}{2}|\uparrow\uparrow\rangle + i\cos\left(\frac{J_x t}{\hbar}\right)\sin\frac{\theta}{2}|\uparrow\downarrow\rangle \\ &+ \sin\left(\frac{J_x t}{\hbar}\right)\sin\frac{\theta}{2}|\downarrow\uparrow\rangle - i\sin\left(\frac{J_x t}{\hbar}\right)\cos\frac{\theta}{2}|\downarrow\downarrow\rangle\Bigg] \,. \end{aligned} \tag{19}$$

This is the final expression of the oscillatory dynamics in global coordinates, using the Zeeman $Z$ basis. In the case where both spins are rotated, the transformations are analogous to:

$$R_1^y(-\theta/2)R_2^y(\theta/2)|\uparrow\uparrow\rangle = R_2^y(\theta/2)R_1^y(-\theta/2)|\uparrow\uparrow\rangle = |\nwarrow\nearrow\rangle \,. \tag{20}$$

Here, only the half spiral angle occurs to guarantee the correct angle between both spins.

## Acknowledgments

R. Wieser acknowledges the financial support provided by the Startup Foundation for Introducing Talent of NUIST (2018r043).

---

[1] A. R. Völkel, F. G. Mertens, A. R. Bishop, and G. M. Wysin, Ann. Phys. **2**, 308 (1993).
